# Supplementary material for: Semantic Importance-Aware Based for Multi-User Communication Over MIMO Fading Channels
Source: arXiv:2312.16057 source file (2023-12-26)
Supplement: Supplementary file 1 [file Appendix.tex]

\section*{Appendix}
